# Supplementary material for: In-plane magnetic structure and exchange interactions in the high-temperature antiferromagnet Cr2Al
Source: arXiv:2201.07356 source file (2022-01-18)
Supplement: Supplementary file 1 [file Supplementary.pdf]

# In-plane magnetic structure and exchange interactions in the high-temperature antiferromagnet $Cr_2Al$

## Supplementary Material

Chengxi Zhao, Kisung Kang, Joerg C. Neuefeind, André Schleife, Daniel P. Shoemaker

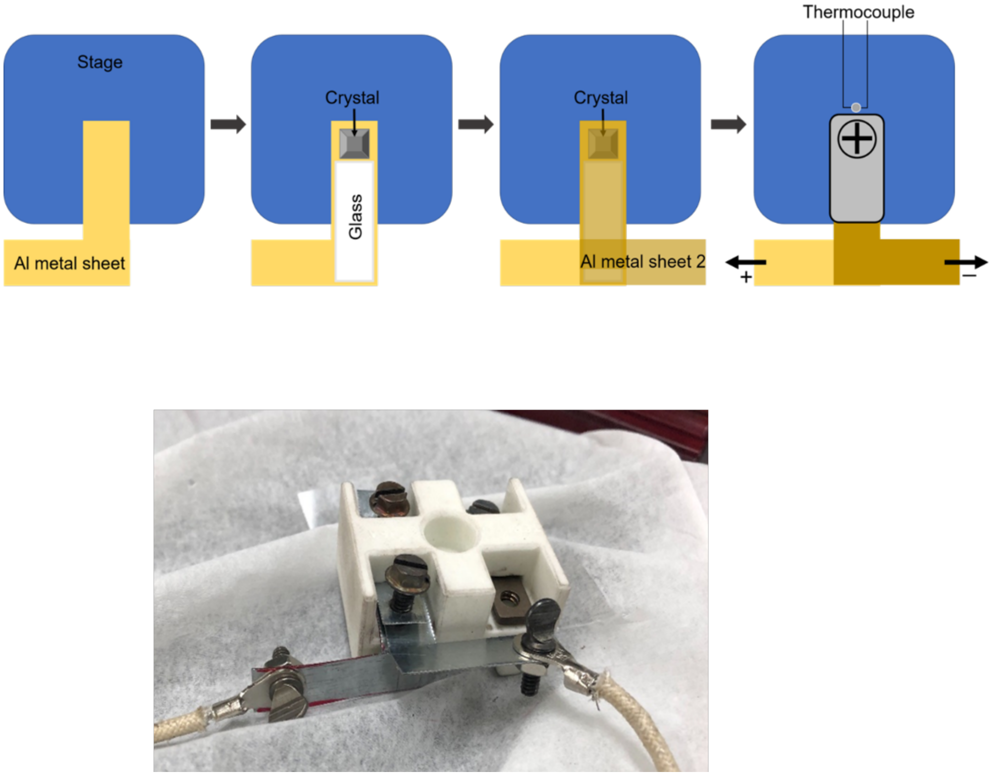


Figure 1: The illustration and picture of the press-contact setup for the two-point resistivity measurement of the single crystal sample.

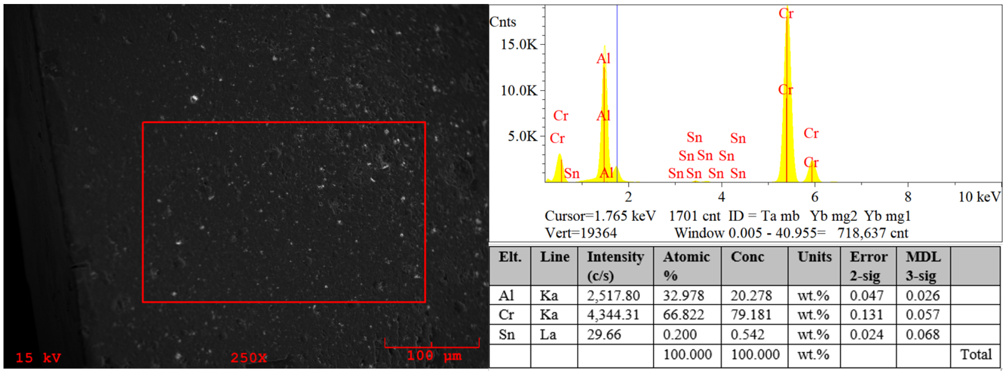


| Elt. | Line | Intensity (c/s) | Atomic % | Conc | Units | Error 2-sig | MDL 3-sig | |
|---|---|---|---|---|---|---|---|---|
| Al | Ka | 2,517.80 | 32.978 | 20.278 | wt.% | 0.047 | 0.026 | |
| Cr | Ka | 4,344.31 | 66.822 | 79.181 | wt.% | 0.131 | 0.057 | |
| Sn | La | 29.66 | 0.200 | 0.542 | wt.% | 0.024 | 0.068 | |
| | | | 100.000 | 100.000 | wt.% | | | Total |

Figure 2: Scanning electron microscope energy-dispersive X-ray spectroscopy measurement of a $Cr_2Al$ single crystal showing elemental molar ratio of Cr:Al to be 2:1.

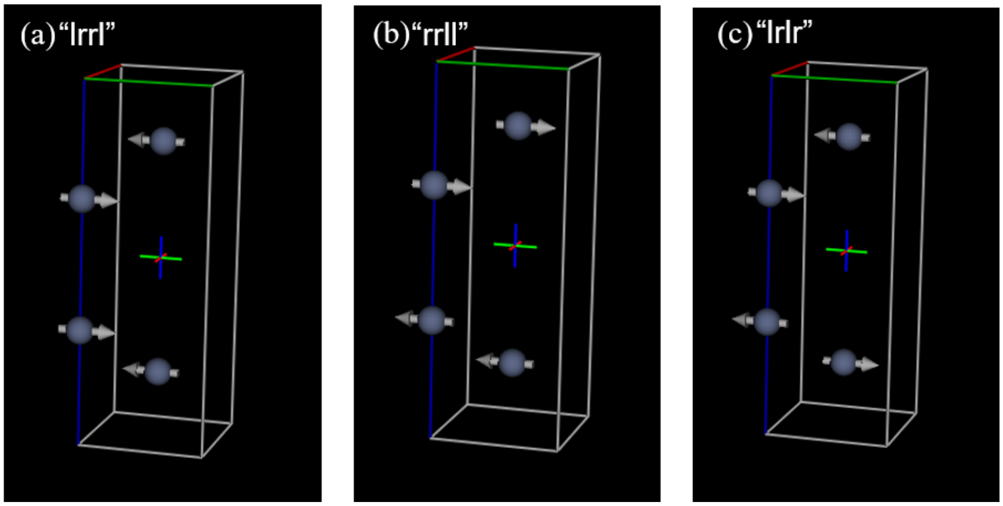


Figure 3: Possible spin arrangements to satisfy antiferromagnetic ordering. The resolved structure from neutron diffraction data is annotated as ”lrrl” because the spins are aligned to ”left-right-right-left” as looking from the top to the bottom of the illustrated structure. The rest of the structures are annotated in the same way.

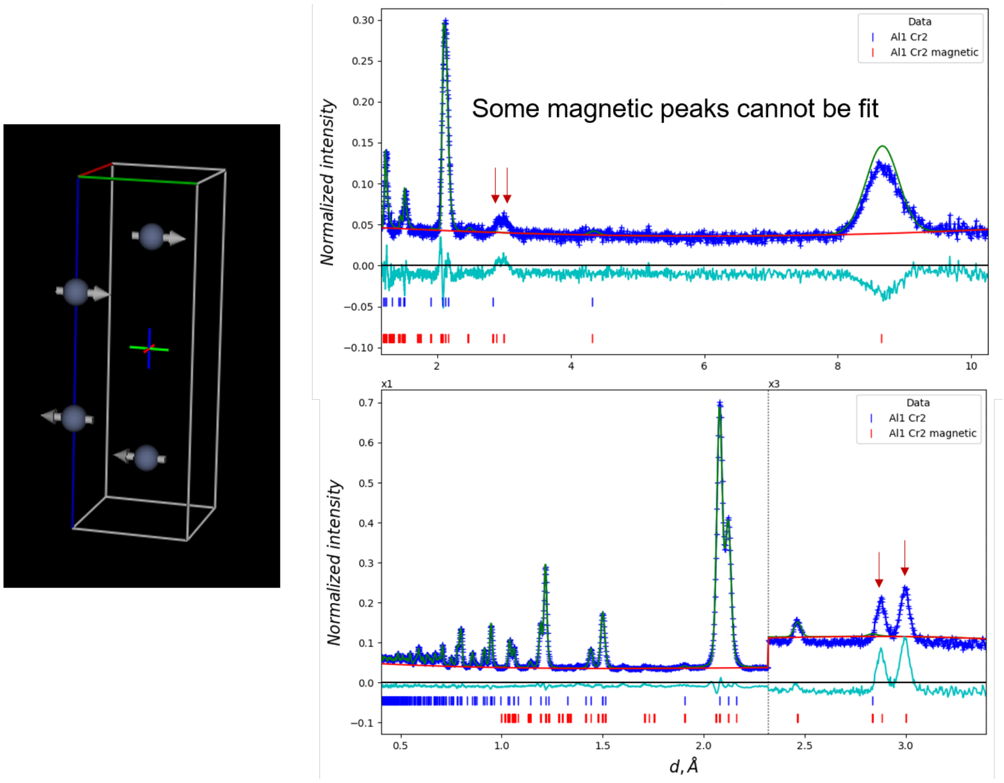


Figure 4: The Rietveld refinement fit of the neutron diffraction pattern with magnetic model constrained as ”rrll” arranged ordering. Some magnetic peaks remained unmatched after refinement.

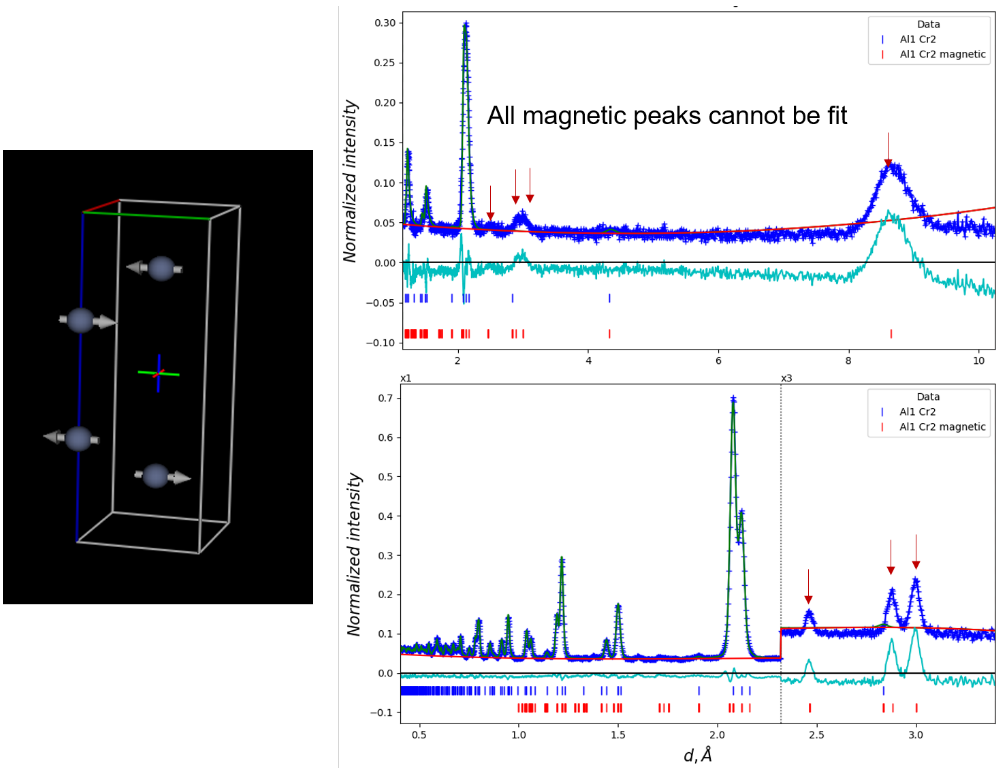


Figure 5: The Rietveld refinement fit of the neutron diffraction pattern with magnetic model constrained as ”lrlr” arranged ordering. All magnetic peaks remained unmatched after refinement.

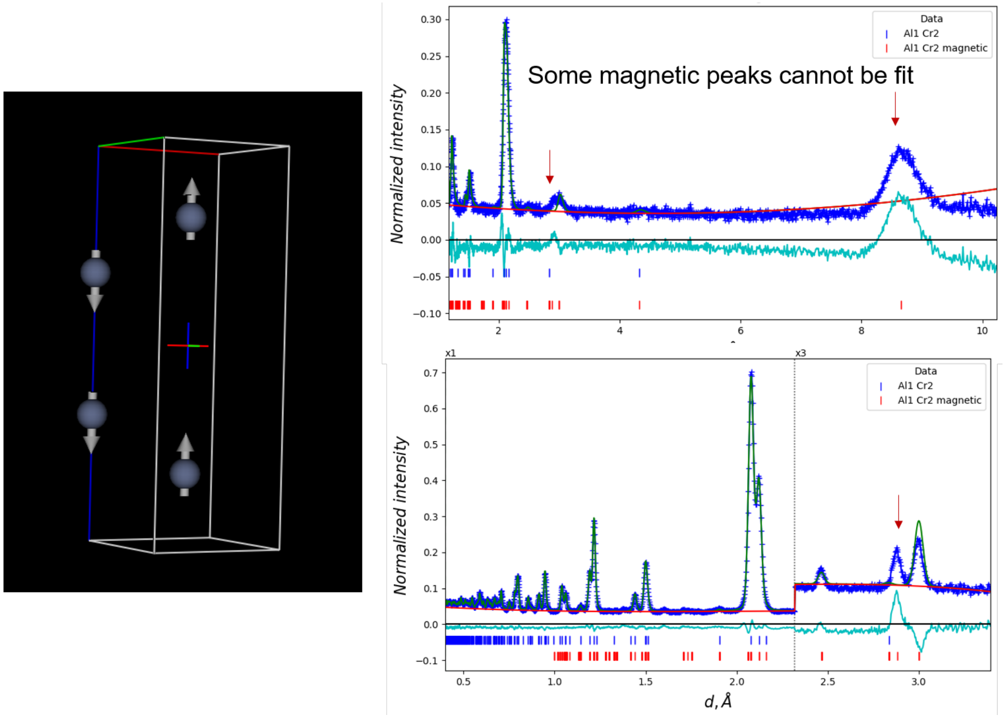


Figure 6: The Rietveld refinement fit of the neutron diffraction pattern with magnetic model constrained as "udud" (up-down-up-down) arranged ordering along c-axis. Some magnetic peaks remained unmatched after refinement.

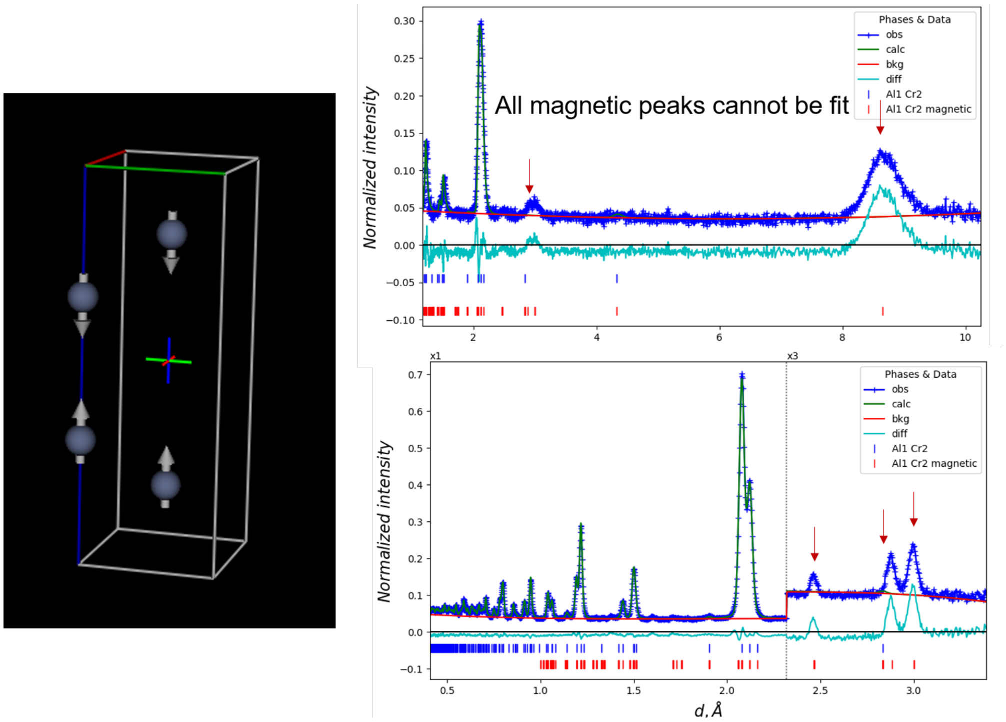


Figure 7: The Rietveld refinement fit of the neutron diffraction pattern with magnetic model constrained as "dduu" (down-down-up-up) arranged ordering along c-axis. All magnetic peaks remained unmatched after refinement.

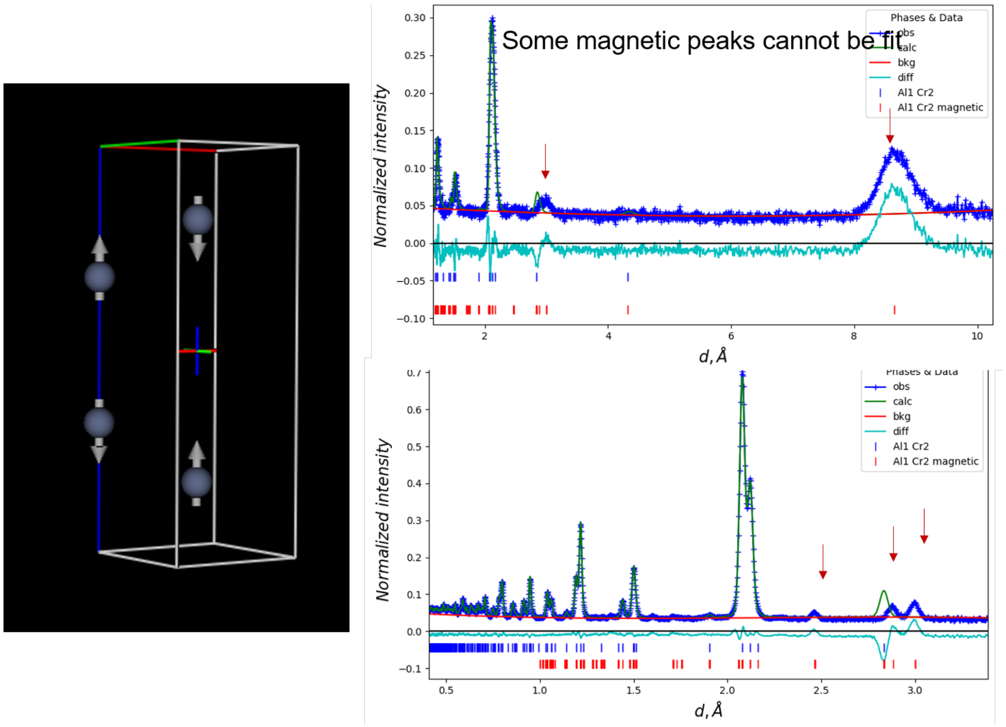


Figure 8: The Rietveld refinement fit of the neutron diffraction pattern with magnetic model constrained as ”dudu” (down-up-down-up) arranged ordering along c-axis. Some magnetic peaks remained unmatched after refinement.

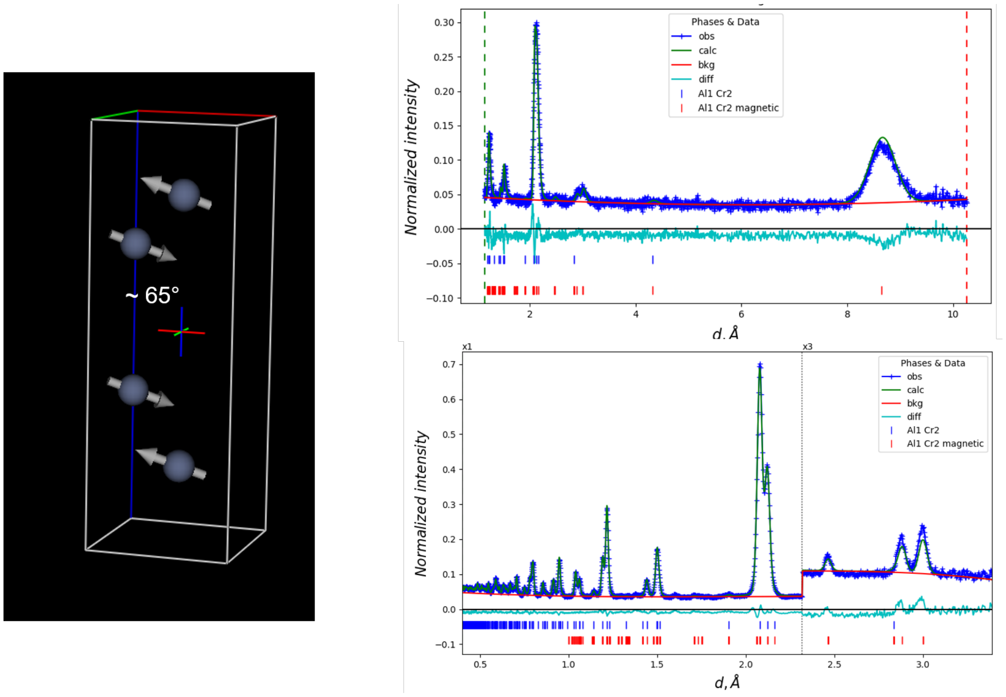


Figure 9: The Rietveld refinement fit of the neutron diffraction pattern with magnetic spins canted as suggested by Atoji. No significant improvement on fitting can be observed.

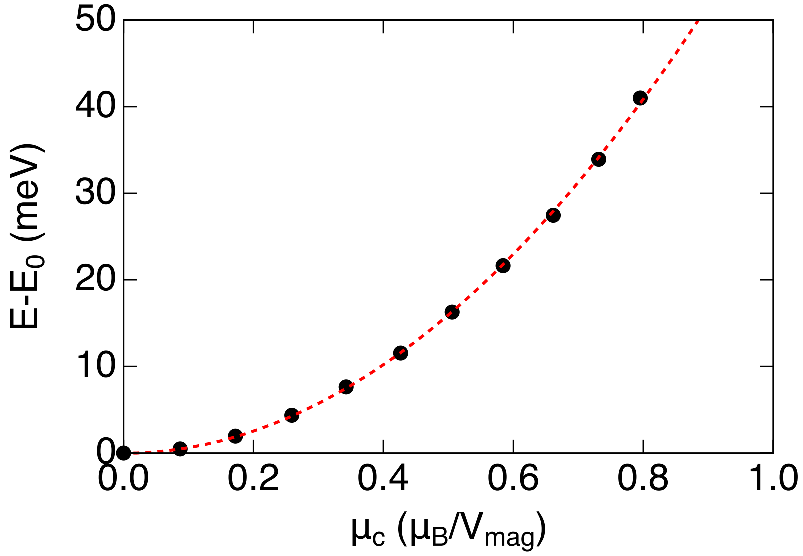


Figure 10: Total energy as a function of net magnetization within magnetic unit cell by changing tilting angle within $ac$-plane from 0° to 10° with a step of 1° (Black circle markers). The red dashed line shows a quadratic fitting curve.

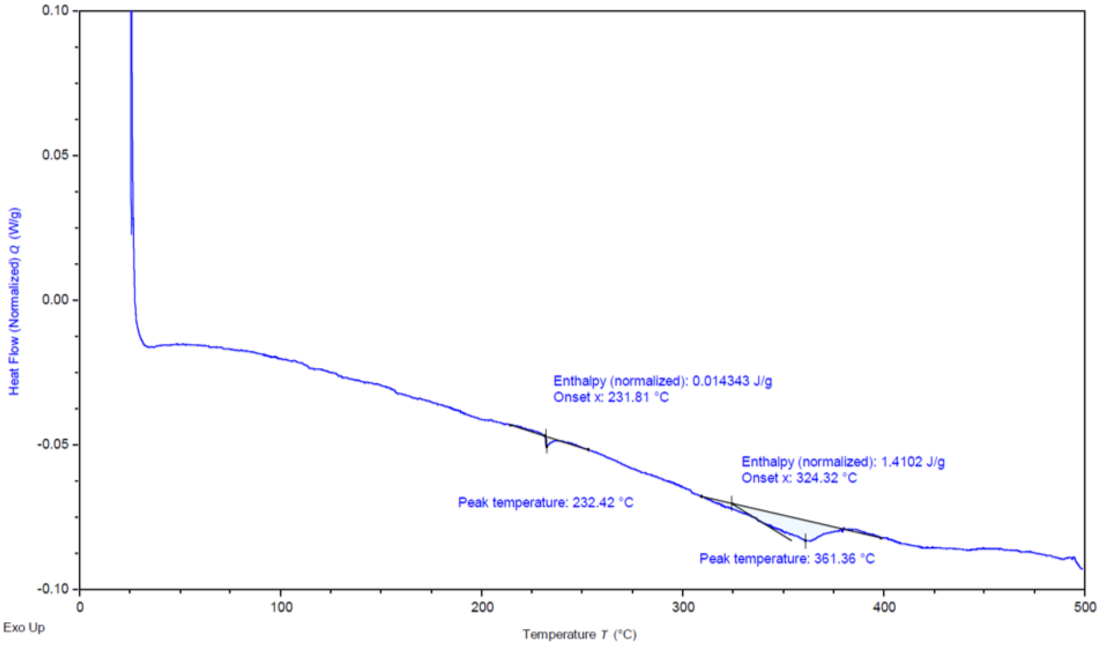


Figure 11: The peak integration analysis of DSC result as shown in Figure 5(b), showing the normalized enthalpy of melting of residual Sn.The enthalpy of melting of Sn is reported to be 7.2 kJ/mol (60.6 J/g) from F. Grønvold, *J. Chem. Thermo.* **25** [9] 1133-1144 (1993).
